# Supplementary material for: PRISM: Progressive Restoration for Scene Graph-based Image Manipulation
Source: arXiv:2311.02247 source file (2023-11-03)
Supplement: Supplementary file 1 [file 6_supplementary.tex]

\section{Architecture Details}
In our work, the decoder generation of manuipulated images is conditioned on the RGB input images as well as the predicted scene layout. During training, the query image corresponds to a masked image. To be specific, we first pass the RGB image through a single layer of 2D convolution. Then, in each residual SPADE block of the the decoder, the shallow feature representation of the masked RGB image is fed alongside the predicted semantic scene layout and the ouput of the previous residual SPADE block as the input. In the first layer, a gaussian noise is used as an input instead of the output from the previous layer. A detailed description of the decoder network alongside the parameters of each layer can seen in~\autoref{tab:detail_decoder}. 

\begin{table*}[ht]
\centering
\begin{tabular}{lllllllll}
Name & Type & In Ch. & Out Ch.  & Filter & Stride & Pad. & Output & Param \\ \Xhline{2pt}  
Inp\_img & DataLayer & - & 4 & - & - & - & $64\times 64$ & - \\
conv\_inp & Convolution & 4 & 32 & $3\times 3$ & 1 & 0 & $64\times 64$ & 160 \\
Scale\_I & Interpolate & 32 & 32 & - & - & - & $4\times 4$ & - \\
Layout & DataLayer & - & 384 & - & - & - & $64\times 64$ & - \\
Scale\_L & Interpolate & 384 & 384 & - & - & - & $4\times 4$ & - \\
Noise & DataLayer & - & 1 & - & - & - & $4\times 4$ & - \\ \hline \hline
SBlk\_0\_0 & SPADE & 384 & 1 & - & - & - & $4\times 4$ & 444K \\
SBlk\_0\_1 & SPADE & 384 & 1 & - & - & - & $4\times 4$ & 444K \\
SBlk\_0\_s & SPADE & 384 & 1 & - & - & - & $4\times 4$ & 444K \\
SBlk\_0\_n0 & Convolution & 33 & 1 & 3 & 1 & 1 & $4\times 4$ & 298 \\
SBlk\_0\_n1 & Convolution & 1 & 1024 & 3 & 1 & 1 & $4\times 4$ & 10K \\
SBlk\_0\_ns & Convolution & 1 & 1024 & 1 & 1 & 0 & $4\times 4$ & 1K \\
SBlk\_1\_0 & SPADE & 384 & 1024 & - & - & - & $8\times 8$ & 2M \\
SBlk\_1\_1 & SPADE & 384 & 512 & - & - & - & $8\times 8$ & 1M \\
SBlk\_1\_s & SPADE & 384 & 1024 & - & - & - & $8\times 8$ & 2M \\
SBlk\_1\_n0 & Convolution & 1056 & 512 & 3 & 1 & 1 & $8\times 8$ & 5M \\
SBlk\_1\_n1 & Convolution & 512 & 512 & 3 & 1 & 1 & $8\times 8$ & 2M \\
SBlk\_1\_ns & Convolution & 1024 & 512 & 1 & 1 & 0 & $8\times 8$ & 500K \\
SBlk\_2\_0 & SPADE & 384 & 512 & - & - & - & $16\times 16$ & 2M \\
SBlk\_2\_1 & SPADE & 384 & 256 & - & - & - & $16\times 16$ & 1M \\
SBlk\_2\_s & SPADE & 384 & 512 & - & - & - & $16\times 16$ & 2M \\
SBlk\_2\_n0 & Convolution & 544 & 256 & 3 & 1 & 1 & $16\times 16$ & 1M \\
SBlk\_2\_n1 & Convolution & 256 & 256 & 3 & 1 & 1 & $16\times 16$ & 590K \\
SBlk\_2\_ns & Convolution & 512 & 256 & 1 & 1 & 0 & $16\times 16$ & 131K \\
SBlk\_3\_0 & SPADE & 384 & 256 & - & - & - & $32\times 32$ & 1M \\
SBlk\_3\_1 & SPADE & 384 & 128 & - & - & - & $32\times 32$ & 737K \\
SBlk\_3\_s & SPADE & 384 & 256 & - & - & - & $32\times 32$ & 1M \\
SBlk\_3\_n0 & Convolution & 288 & 128 & 3 & 1 & 1 & $32\times 32$ & 331K \\
SBlk\_3\_n1 & Convolution & 128 & 128 & 3 & 1 & 1 & $32\times 32$ & 147K \\
SBlk\_3\_ns & Convolution & 256 & 128 & 1 & 1 & 0 & $32\times 32$ & 33K \\
SBlk\_4\_0 & SPADE & 384 & 128 & - & - & - & $64\times 64$ & 737K \\
SBlk\_4\_1 & SPADE & 384 & 64 & - & - & - & $64\times 64$ & 590K \\
SBlk\_4\_s & SPADE & 384 & 128 & - & - & - & $64\times 64$ & 737K \\
SBlk\_4\_n0 & Convolution & 160 & 64 & 3 & 1 & 1 & $64\times 64$ & 92K \\
SBlk\_4\_n1 & Convolution & 64 & 64 & 3 & 1 & 1 & $64\times 64$ & 37K \\
SBlk\_4\_ns & Convolution & 128 & 64 & 1 & 1 & 0 & $64\times 64$ & 8K \\ \hline \hline
out\_conv & Convolution & 64 & 64 & $3\times 3$ & 1 & 1 & $64\times 64$  & 37K  \\
out\_conv & LeakyReLu & - & - & - & - & - & $64\times 64$ & -0.2  \\
out\_conv & Convolution  & 64 & 3 & $1\times 1$ & 1 & 0 & $64\times 64$  & 195 \\
out\_conv2 & Convolution  & 67 & 64 & $3\times 3$ & 1 & 1 & $64\times 64$ & 39K \\
out\_conv2 & LeakyReLu & - & - & - & - & - & $64\times 64$ & -0.2 \\
out\_conv2 & Convolution  & 64 & 3 & $1\times 1$ & 1 & 0 & $64\times 64$ & 195
\end{tabular}
\caption[Detailed desicription of the decoder architecture]{Detailed description of the decoder archtecture parameters. \textbf{Param}: describes either the number of paramters of the layer or a function parameter depending on the type of the layer, \textbf{SBlk}: Spade Resnet block, \textbf{Ch.}: Channel, \textbf{Pad.}: Padding}\label{tab:detail_decoder}
\end{table*}

\section{Additional Qualitative Results}
\begin{figure}[ht]
    \centering
    \includegraphics[width=0.45\textwidth]{figures/appendix3_magnified_publication.pdf}
    \caption[Ground-truth CLEVR image sample alongside the predicted output of two-headed approach]{An example of a ground-truth CLEVR image sample \textbf{(left)}, entire image reconstruction prediction from the first head of the two-headed approach \textbf{(middle)}, and a detailed reconstruction of the previously masked image by the second head \textbf{(right)}}\label{fig:comparison_two_head_baseline_gt}
\end{figure}

\begin{figure*}[ht]
    \centering
    \includegraphics[width=0.9\textwidth]{figures/SIMSG_vs_PRISM_VG_all3_modes_appendix1_publication.pdf}
    \caption[Qualitative comparison between SIMSG and PRISM on VG dataset]{Qualitative comparison between SIMSG~\cite{simsg} and PRISM on VG~\cite{VG_2017} dataset}
    \label{fig:appendix_qual1}%
\end{figure*}

\begin{figure*}[ht]
    \centering
    \includegraphics[width=0.9\textwidth]{figures/SIMSG_vs_PRISM_VG_all3_modes_appendix2_publication.pdf}
    \caption[Qualitative comparison between SIMSG and PRISM on VG dataset]{Qualitative comparison between SIMSG~\cite{simsg} and PRISM on VG~\cite{VG_2017} dataset}
    \label{fig:appendix_qual1}%
\end{figure*}
